# Supplementary material for: Kick Back & Relax: Learning to Reconstruct the World by Watching SlowTV
Source: arXiv:2307.10713 source file (2023-07-20)
Supplement: Supplementary file 1 [file supp_preds_fail.tex]

% Zero-shot depth estimation failure cases.

\def\w{0.103}

\def\datas{
    img/Image
    ,depth/GT
}

\def\selfsup{
    % ,garg/Garg~\cite{Garg2016}
    % ,monodepth2_MS/Monodepth2~\cite{Godard2019}
    hrdepth_MS/HR-Depth
    ,base/Ours
}

\def\sup{
    MiDaS/MiDaS
    % ,DPT_Large/DPT-ViT~\cite{Ranftl2021}
    ,DPT_BEiT_L_512/DPT-BEiT
    ,newcrfs/NeWCRFs
}

\def\nums{
    viz_base/kitti_eigen_benchmark_0234%
    ,viz_zero_out/syns_test_0026%
    ,viz_zero_out/sintel_0086%
    ,viz_base/mc_0513%
    ,viz_zero_out/ddad_0521%
    ,viz_zero_out/diode_outdoor_0336%
    ,viz_zero_in/diode_indoors_0110%
    ,viz_zero_in/nyud_0055%
    ,viz_zero_in/tum_0668%
}

\def\ds{
    Kitti
    ,SYNS
    ,Sintel
    ,Mannequin
    ,DDAD
    ,Diode
    ,Diode
    ,NYUD
    ,TUM
}

\def\divider{\textcolor{black}{\hdashrule[2mm][x]{\linewidth}{\heavyrulewidth}{2pt}}}

\noindent
\rotatebox{90}{\color{white}{\textbf{\scriptsize Tmp}}}
\foreach \d in \ds{\makebox[\w\linewidth][c]{\textbf{\scriptsize\d}}\hfill}

\foreach \method/\label in \datas{%
    \rotatebox{90}{\textbf{\scriptsize \label}}
    \foreach \num in \nums{% 
        \includegraphics[width=\w\linewidth]{\num_\method}\hfill%
    } \\
}

\divider

\foreach \method/\label in \selfsup{%
    \rotatebox{90}{\textbf{\scriptsize \label}}
    \foreach \num in \nums{% 
        \includegraphics[width=\w\linewidth]{\num_\method}\hfill%
    } \\
}

\divider

\foreach \method/\label in \sup{%
    \rotatebox{90}{\textbf{\scriptsize \label}}
    \foreach \num in \nums{% 
        \includegraphics[width=\w\linewidth]{\num_\method}\hfill%
    } \\
}

\mycaption{Failure Cases}{%
The proposed model occasionally produces holes of infinite depth or texture-copy artefacts. 
However, complex regions such as foliage or boundaries tend to be oversmoothed by all approaches. 
Finally, the upright prior in training data makes the model less robust to strong rotations. 
\emph{Middle=Self-Supervised -- Bottom=Supervised.}
}
