# Supplementary material for: Kick Back & Relax: Learning to Reconstruct the World by Watching SlowTV
Source: arXiv:2307.10713 source file (2023-07-20)
Supplement: Supplementary file 2 [file supp_res.tex]

% Supplementary results using median scaling. 

\addtolength{\tabcolsep}{0.2em}
\def\mc{\multicolumn}

\mycaption{Median-Scaling Results}{%
This represents the common \ac{ssmde} evaluation procedure~\cite{Zhou2017}. 
Removing the shift alignment reduces performance for all approaches. 
Our method still outperforms all existing \acl{ssmde} models, and \ac{crf} in many cases.
}

\begin{tabular}{@{}llllllllllllllllllll@{}}
\toprule
                             &       & \mc{4}{c}{\bf In-Distribution}                                         & \mc{8}{c}{\bf Outdoor}                                                                                                        & \mc{6}{c}{\bf Indoor}                                                                            \\
                                       \cmidrule(lr){3-6}                                                       \cmidrule(lr){7-14}                                                                                                             \cmidrule(lr){15-20}
                             &       & \mc{2}{c}{\bf\acs{keb}}            & \mc{2}{c}{\bf\acs{mc}}            & \mc{2}{c}{\bf\acs{ddad}}      & \mc{2}{c}{\bf\acs{dio}}       & \mc{2}{c}{\bf\acs{sintel}}    & \mc{2}{c}{\bf\acs{syns}}      & \mc{2}{c}{\bf\acs{dii}}       & \mc{2}{c}{\bf\acl{nyud}}         & \mc{2}{c}{\bf\acs{tum}}       \\  
                                       \cmidrule(lr){3-4}                   \cmidrule(lr){5-6}                  \cmidrule(lr){7-8}              \cmidrule(lr){9-10}             \cmidrule(lr){11-12}            \cmidrule(lr){13-14}            \cmidrule(lr){15-16}            \cmidrule(lr){17-18}               \cmidrule(lr){19-20}
                             & Train &        Rel\down &             F\up &        Rel\down &            F\up &      Rel\down &          F\up &      Rel\down &  \acs{d25}\up &      Rel\down &          F\up &      Rel\down &          F\up &      Rel\down &  \acs{d25}\up &       Rel\down &    \acs{d25}\up &      Rel\down &  \acs{d25}\up \\
\midrule
Garg~\cite{Garg2016}         & S     & \zs\nbest{7.65} & \zs\nbest{53.28} & \nbest{34.55} & \nbest{9.29} &         26.77 &         4.77 &         57.87 &             42.85 & \nbest{53.16} & \nbest{30.98} &         31.68 &         13.58 &         30.63 &             51.00 &         26.78 &             54.29 & \nbest{27.37} &     \nbest{55.26} \\
Monodepth2~\cite{Godard2019} & MS    &  \zs       7.90 &   \zs      50.50 &         35.88 &         8.18 &         25.46 &         4.77 &         57.61 &             43.21 &         54.40 &         30.11 &         30.05 &         13.28 &         33.51 &             47.49 &         29.87 &             50.08 &         30.59 &             49.82 \\
DiffNet~\cite{Zhou2021}      & MS    &  \zs       7.98 &   \zs      49.60 &         35.50 &         8.15 &         24.17 &         4.75 & \nbest{55.68} &     \nbest{45.37} &         55.23 &         29.44 & \nbest{29.75} &         13.41 & \nbest{28.67} &     \nbest{53.82} & \nbest{26.62} &     \nbest{54.69} &         28.56 &             53.07 \\
HR-Depth~\cite{Lyu2021}      & MS    &  \zs       7.70 &   \zs      51.49 &         35.89 &         8.62 & \nbest{24.01} & \nbest{5.08} &         57.88 &             43.92 &         53.91 &         30.89 &         29.87 & \nbest{14.03} &         32.88 &             47.67 &         27.32 &             53.06 &         29.22 &             52.31 \\
\midrule
\textbf{\acs{kbr} (Ours)}    & M     &  \zs\best{7.23} &  \zs\best{54.63} &  \zs\best{18.73} & \zs\best{15.04} &  \best{14.01} & \best{14.01} &  \best{43.80} &      \best{60.84} &  \best{37.06} &  \best{36.01} &  \best{24.92} &  \best{16.49} &  \best{18.88} &      \best{72.09} &  \best{13.27} &      \best{83.65} &  \best{16.60} &      \best{76.48} \\
\midrule
\midrule
MiDaS~\cite{Ranftl2020}      & D     &         18.45 &         20.13 & \nbest{26.02} &         10.61 &         18.38 &          8.28 &  \best{48.63} &      \best{60.15} &  \best{39.09} &  \best{32.72} &         35.30 &          9.18 & \nbest{18.08} &     \nbest{74.48} & \nbest{23.11} &     \nbest{69.67} & \nbest{17.75} &             76.99 \\ 
DPT-ViT~\cite{Ranftl2021}    & D     & \nbest{14.23} &         36.25 &         28.54 &         11.38 &         17.83 &          8.99 &         72.46 &             49.09 &        128.86 &         29.58 &         32.69 &         12.93 &         36.82 &             55.15 &         24.82 &             67.95 &         24.33 &             78.16 \\ 
DPT-BEiT~\cite{Ranftl2021}   & D     &  \zs       18.20 & \zs\nbest{37.46} &         30.79 & \nbest{12.58} & \nbest{15.39} & \nbest{11.78} &         70.30 &             50.03 &         60.20 &         29.54 & \nbest{31.09} & \nbest{13.76} &         51.07 &             53.11 &    \zs     75.32 &   \zs          42.91 &         25.27 &      \best{83.07} \\ 
NeWCRFs~\cite{Weihao2022}    & D     &  \zs \best{5.55} & \zs \best{56.45} &  \best{22.15} &  \best{13.68} &  \best{11.87} &  \best{13.44} & \nbest{50.52} &     \nbest{51.16} & \nbest{48.42} & \nbest{32.30} &  \best{27.79} &  \best{14.50} &  \best{16.15} &      \best{79.52} &   \zs\best{7.00} &   \zs   \best{94.44} &  \best{14.93} &     \nbest{80.63} \\ 
\bottomrule
\end{tabular}

\emph{%
Highlighted cells are \emph{\textbf{NOT zero-shot}} results.
\textbf{S}=Stereo, \textbf{M}=Monocular, \textbf{D}=Ground-truth Depth.
}
