# Supplementary material for: Kick Back & Relax: Learning to Reconstruct the World by Watching SlowTV
Source: arXiv:2307.10713 source file (2023-07-20)
Supplement: Supplementary file 3 [file supp_preds_motion.tex]

% Zero-shot depth estimation failure cases.

\def\w{0.2}

\def\datas{
    img/Image
    ,depth/GT
}

\def\models{
    full_no_md2_042/Baseline
    ,full_md2_042/Monodepth2
}

\def\nums{
    viz_motion/kitti_eigen_benchmark_0408%
    ,viz_motion/ddad_0973%
    ,viz_motion/sintel_0570%
    ,viz_motion/tum_1064%
}

\foreach \method/\label in \datas{%
    \rotatebox{90}{\textbf{\scriptsize \label}}
    \foreach \num in \nums{% 
        \includegraphics[width=\w\linewidth]{\num_\method}\hfill%
    } \\
}

\foreach \method/\label in \models{%
    \rotatebox{90}{\textbf{\scriptsize \label}}
    \foreach \num in \nums{% 
        \includegraphics[width=\w\linewidth]{\num_\method}\hfill%
    } \\
}

\mycaption{Monodepth2 Losses}{%
Monodepth2~\cite{Godard2019} reduces the presence of holes of infinite depth and dynamic object artefacts. 
The sharpness of object boundaries are also improved due to the refined correspondences from the minimum reconstruction loss. 
}
